# Supplementary material for: GlobeDiff: State Diffusion Process for Partial Observability in Multi-Agent Systems
Source: arXiv:2602.15776 source file (2026-02-17)
Supplement: Supplementary file 1 [file add_exp.tex]

\clearpage
\section{Additional Experiments}

\begin{figure*}[t]
    \centering
    \subfigure{\includegraphics[scale=0.25]{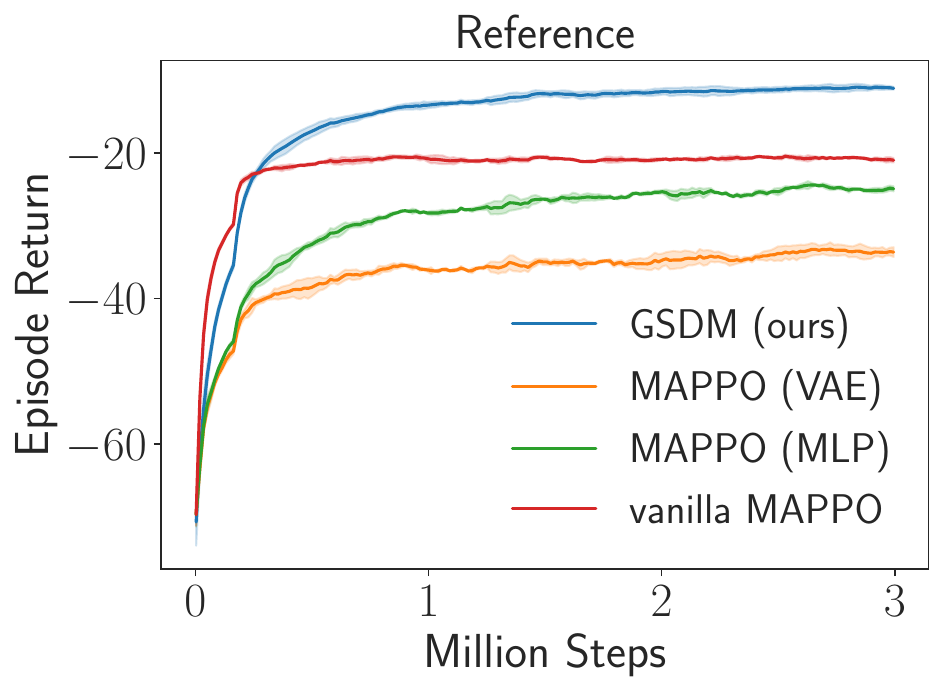}}
    \subfigure{\includegraphics[scale=0.25]{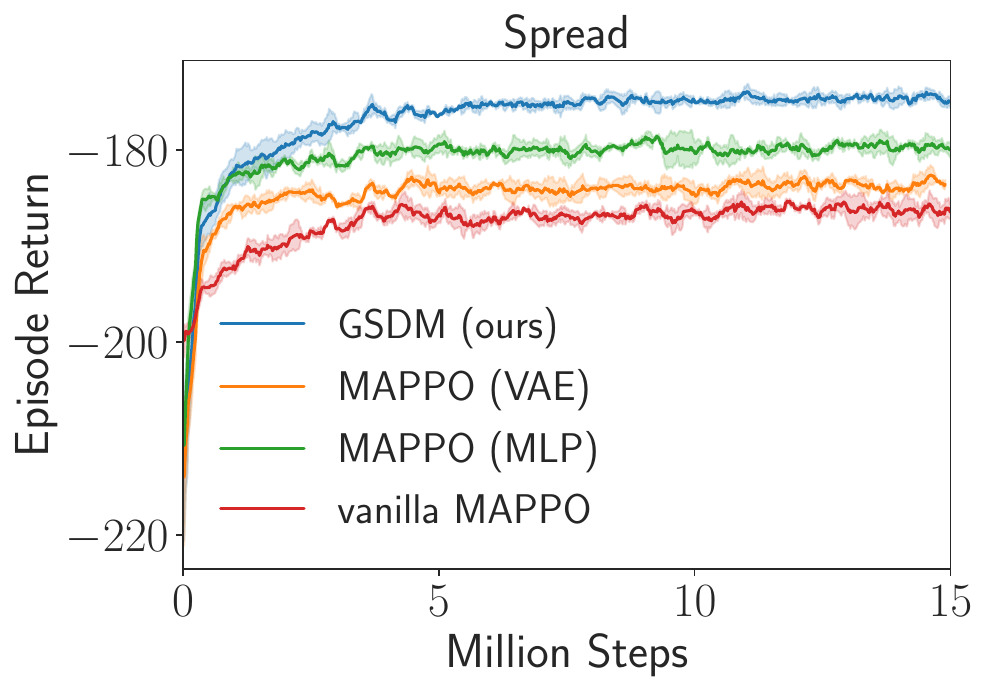}}
    \subfigure{\includegraphics[scale=0.25]{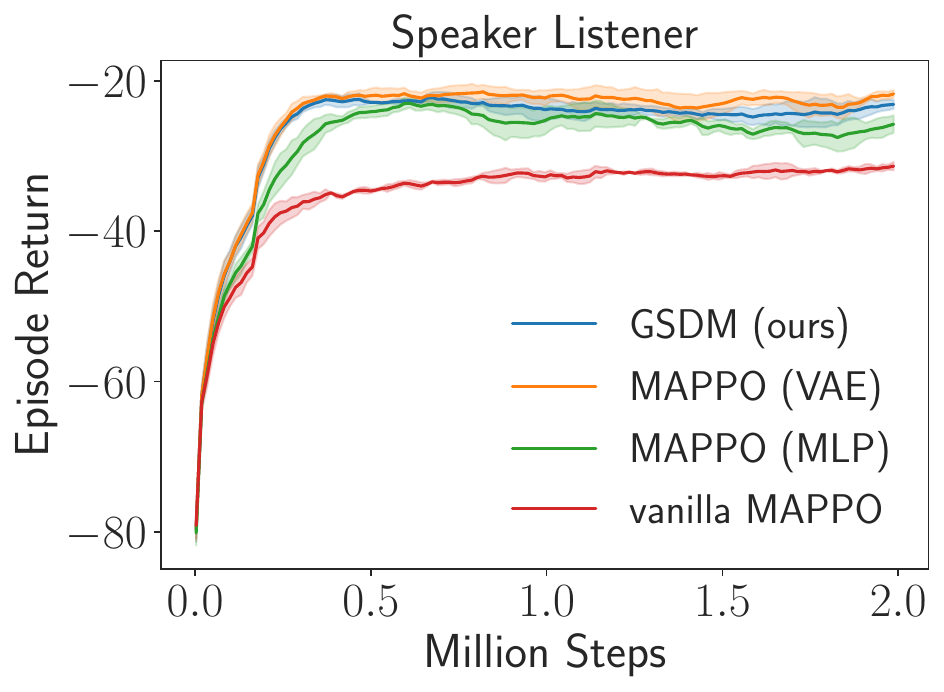}}
    \caption{Experimental results for MPE tasks with episode return averaged with three random seeds.}
    \label{fig: mpe}
\end{figure*}

\begin{figure}[t]
    \centering
    \subfigure{\includegraphics[scale=0.35]{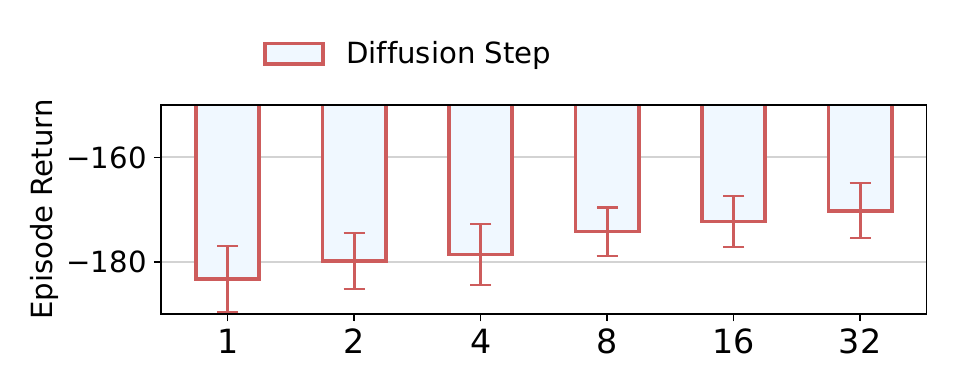}}
    \includegraphics[scale=0.35]{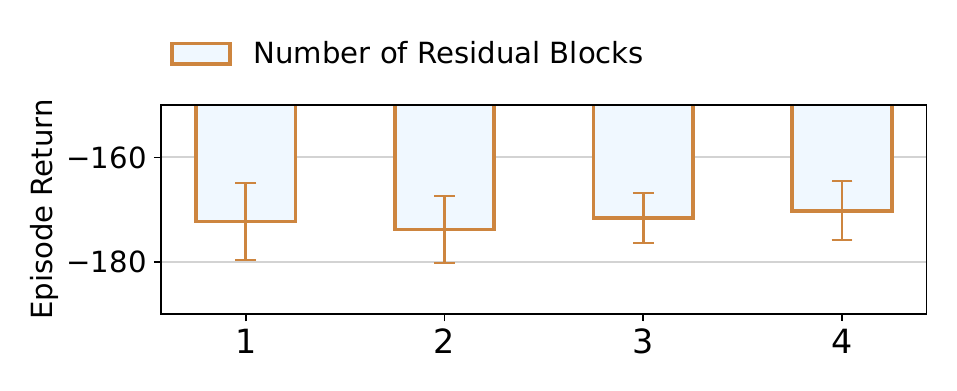}
    \caption{Ablation study on the Spread task in MPE with various diffusion steps $K$.}
    \label{fig: ablation step}
\end{figure}

We conduct additional comparison with baselines.
Specifically, we compare our method with generative model-based methods GAN~\citep{goodfellow2014generative} and value function decomposition methods (QPLEX~\citep{wang2020qplex}) in SMAC. 
Further, we compare our method with GAN, MADDPG~\citep{lowe2017multi} and its variants (MAAC~\citep{iqbal2019actor}) in the MPE scenario. 
The experimental results in Table~\ref{table: add-smac-v1} show that GlobeDiff outperforms both GAN and QPLEX across all SMAC maps. For instance, in the challenging 6h-vs-8z scenario, GlobeDiff achieves a 72\% higher success rate than QPLEX.
For the MPE tasks, the experimental results in Table~\ref{table: add-mpe} show that GlobeDiff surpasses MADDPG, MAAC, and GAN in all tasks. For example, in the Speaker Listener task, GlobeDiff achieves an episode return of -22.6, significantly better than MAAC (-30.6) and MADDPG (-32.4).

\begin{table*}[h]
\begin{center}
    \begin{tabular}{l|c|c|c|c} 
    \toprule
      Tasks & BAD & GAN & QPLEX & GlobeDiff \\
      \midrule
      MMM2 & 0.375$\pm$0.048 & 0.324$\pm$0.045 & 0.286$\pm$0.047 & 0.492$\pm$0.052 \\
      6h-vs-8z & 0.289$\pm$0.045 & 0.268$\pm$0.041 & 0.175$\pm$0.042 & 0.479$\pm$0.036 \\
      3s5z-vs-3s6z & 0.184$\pm$0.033 & 0.174$\pm$0.036 & 0.162$\pm$0.032 & 0.286$\pm$0.034 \\
      \bottomrule
    \end{tabular}
\end{center}
\caption{Experimental results for SMAC-v1 tasks with success rate metric averaged with three
random seeds.}
\label{table: add-smac-v1}
\end{table*}

\begin{table*}[h]
\begin{center}
    \begin{tabular}{l|c|c|c|c} 
    \toprule
      Tasks & GAN & MADDPG & MAAC & GlobeDiff\\
      \midrule
      Reference & -23.4$\pm$0.3 & -25.1$\pm$0.2 & -20.3$\pm$0.3 & -10.4$\pm$0.2 \\
      Spread & -182.4$\pm$3.5 & -189.4$\pm$4.2 & -187.5$\pm$3.1 & -176.2$\pm$3.2 \\
      Speaker Listener & -24.8$\pm$1.3 & -32.4$\pm$1.4 & -30.6$\pm$1.5 & -22.6$\pm$1.5 \\
      \bottomrule
    \end{tabular}
\end{center}
\caption{Experimental results for MPE tasks with episode return metric averaged with three random
seeds.}
\label{table: add-mpe}
\end{table*}

We conduct additional ablation studies by changing historical steps from 1 to 5 in the diffusion model.
The experimental results in Table~\ref{table: historical} show that the diffusion model effectively integrates historical information to infer latent global states.

\begin{table*}[h]
\begin{center}
    \begin{tabular}{l|c|c|c|c} 
    \toprule
      Historical Steps & 1 & 2 & 3 & 5 \\
      \midrule
      MMM2 & 0.385$\pm$0.044 & 0.444$\pm$0.052 & 0.492$\pm$0.052 & 0.498$\pm$0.051 \\
      6h-vs-8z & 0.378$\pm$0.035 & 0.456$\pm$0.035 & 0.479$\pm$0.036 & 0.483$\pm$0.033 \\
      3s5z-vs-3s6z & 0.184$\pm$0.034 & 0.243$\pm$0.036 & 0.286$\pm$0.034 & 0.289$\pm$0.031 \\
      \bottomrule
    \end{tabular}
\end{center}
\caption{Ablation study on the SMAC-v1 tasks with various historical steps.}
\label{table: historical}
\end{table*}

\clearpage

In addition, we conduct additional ablation studies in SMAC by changing diffusion steps K from 1 to 32.
The experimental results in Table~\ref{table: diffusion step} show that the performance improves as K increases.
However, larger K incurs higher computational costs. 
We chose K=5 as a balance between performance and efficiency.
We extended ablation studies to SMAC to assess the impact of residual blocks.
The experimental results in Table~\ref{table: residual blocks} show that using 2 blocks achieves the best performance (e.g., 0.438 in 6h-vs-8z), while increasing blocks degrades results due to overfitting. This confirms that a lightweight architecture suffices for state inference.

\begin{table*}[h]
\begin{center}
    \begin{tabular}{l|c|c|c|c|c} 
    \toprule
      Diffusion Steps & 1 & 2 & 5 & 16 & 32 \\
      \midrule
      MMM2 & 0.431$\pm$0.049 & 0.470$\pm$0.048 & 0.492$\pm$0.052 & 0.494$\pm$0.051 & 0.495$\pm$0.050 \\
      6h-vs-8z & 0.431$\pm$0.037 & 0.458$\pm$0.031 & 0.479$\pm$0.036 & 0.483$\pm$0.034 & 0.484$\pm$0.035 \\
      3s5z-vs-3s6z & 0.225$\pm$0.037 & 0.262$\pm$0.031 & 0.286$\pm$0.034 & 0.287$\pm$0.032 & 0.289$\pm$0.030 \\
      \bottomrule
    \end{tabular}
\end{center}
\caption{Ablation study on the SMAC-v1 tasks with various diffusion steps.}
\label{table: diffusion step}
\end{table*}

\begin{table*}[h]
\begin{center}
    \begin{tabular}{l|c|c|c|c} 
    \toprule
      Residual Blocks & 1 & 2 & 3 & 4 \\
      \midrule
      MMM2 & 0.479$\pm$0.047 & 0.492$\pm$0.052 & 0.494$\pm$0.051 & 0.493$\pm$0.053 \\
      6h-vs-8z & 0.465$\pm$0.034 & 0.479$\pm$0.036 & 0.481$\pm$0.037 & 0.478$\pm$0.034 \\
      3s5z-vs-3s6z & 0.277$\pm$0.032 & 0.286$\pm$0.034 & 0.285$\pm$0.035 & 0.284$\pm$0.033\\
      \bottomrule
    \end{tabular}
\end{center}
\caption{Ablation study on the SMAC-v1 tasks with various residual blocks.}
\label{table: residual blocks}
\end{table*}

\paragraph{Computationtal Cost}
We conduct experiments on the A100 GPU device. 
In the SMAC-V1 environment and SMAC-V2 environment, our algorithm takes an average of 28 hours and 30 hours to run to 10M steps, respectively.
