# Supplementary material for: GlobeDiff: State Diffusion Process for Partial Observability in Multi-Agent Systems
Source: arXiv:2602.15776 source file (2026-02-17)
Supplement: Supplementary file 2 [file proof.tex]

\section{MATHEMATICAL DERIVATIONS}
\newtheorem*{reptheorem}{Theorem}
% \newtheorem{appendixtheorem}{Theorem}[section]
% \renewcommand{\theappendixtheorem}{A.\arabic{appendixtheorem}}

% \subsection{Problem Setup}
% Let the global state \( s \in \mathbb{R}^d \) follow a distribution \( p(s) \), with partial observation \( x = Ms + \eta \), where \( M \in \mathbb{R}^{m \times d} \) (\( m < d \)) and \( \eta \sim \mathcal{N}(0, \sigma^2 I) \). The goal is to sample from \( p(s|x) \) using a diffusion model with MSE loss for noise prediction.

\subsection{Error Bound Analysis for Single Samples}
\label{proof:single}
\begin{reptheorem}[Theorem~\ref{thm:single} (Single-Sample Expectation Error Bound)]

% \begin{theorem}[Single-Sample Expectation Error Bound]
% \label{thm:single}

Assume the trained model satisfies \( \mathbb{E}[\| \epsilon_\theta - \epsilon \|^2] \leq \delta^2 \). For any generated sample \( \hat{s} \sim p_\theta(s|x) \) and true sample \( s \sim p(s|x) \), the expected squared error is bounded by:
\begin{equation}
    \mathbb{E}\left[ \| \hat{s} - s \|^2 \right] \leq 2W_2^2(p_\theta(s|x), p(s|x)) + 2\text{Var}(s|x),
\end{equation}

where:
\begin{itemize}
\item \( W_2 \) is the 2-Wasserstein distance between \( p_\theta(s|x) \) and \( p(s|x) \),
\item \( \text{Var}(s|x) = \mathbb{E}_{p(s|x)}\left[\| s - \mu_{s|x} \|^2\right] \) is the conditional variance,
\item \( \mu_{s|x} = \mathbb{E}_{p(s|x)}[s] \) is the conditional mean.
\end{itemize}
% \end{theorem}
\end{reptheorem}

\begin{proof}
\textbf{Step 1: Error Decomposition via Variance-Bias Tradeoff}\\
Let \( \mu_{s|x} = \mathbb{E}_{p(s|x)}[s] \). For any \( \hat{s} \) and \( s \), we can expand the squared error as:
\begin{equation}
\| \hat{s} - s \|^2 = \| (\hat{s} - \mu_{s|x}) - (s - \mu_{s|x}) \|^2.
\end{equation}
By applying the Cauchy-Schwarz inequality:
\begin{equation}
\| a - b \|^2 \leq 2\|a\|^2 + 2\|b\|^2,
\end{equation}
we obtain:
\begin{equation}
\mathbb{E}\left[\| \hat{s} - s \|^2\right] \leq 2\mathbb{E}\left[\| \hat{s} - \mu_{s|x} \|^2\right] + 2\mathbb{E}\left[\| s - \mu_{s|x} \|^2\right].
\end{equation}

\textbf{Step 2: Bounding the First Term via Wasserstein Distance}

% \begin{enumerate}
% \item Variance-Bias Decomposition

For any generated sample \( \hat{s} \sim p_\theta(s|x) \), we can decompose the squared deviation from the true conditional mean \( \mu_{s|x} \) as:
\begin{equation}
\mathbb{E}\left[\| \hat{s} - \mu_{s|x} \|^2\right] = \underbrace{\mathbb{E}\left[\| \hat{s} - \mu_{p_\theta} \|^2\right]}_{\text{Generated Variance}} + \underbrace{\| \mu_{p_\theta} - \mu_{s|x} \|^2}_{\text{Bias}^2},
\end{equation}
where \( \mu_{p_\theta} = \mathbb{E}_{p_\theta}[\hat{s}] \) is the mean of the generated distribution.

% \item Link to Wasserstein Distance

The Wasserstein-2 distance between \( p_\theta \) and \( p(s|x) \) inherently controls both variance and bias components:
\begin{equation}
W_2^2(p_\theta, p) = \inf_{\gamma \in \Gamma(p_\theta, p)} \mathbb{E}_{(\hat{s}, s) \sim \gamma} \left[\| \hat{s} - s \|^2\right].
\end{equation}
For any coupling \( \gamma \), the squared distance can be expanded as:
\begin{equation}
\mathbb{E}_\gamma\left[\| \hat{s} - s \|^2\right] = \mathbb{E}\left[\| \hat{s} - \mu_{p_\theta} \|^2\right] + \mathbb{E}\left[\| s - \mu_{s|x} \|^2\right] + \| \mu_{p_\theta} - \mu_{s|x} \|^2.
\end{equation}
Taking the infimum over all couplings \( \gamma \), we obtain:
\begin{equation}
W_2^2(p_\theta, p) \leq \text{Var}(p_\theta) + \text{Var}(s|x) + \| \mu_{p_\theta} - \mu_{s|x} \|^2.
\end{equation}

% \item Optimal Transport Alignment

Under the optimal transport plan that minimizes the Wasserstein distance, the following two conditions can be satisfied:
1. Mean Alignment: The optimal coupling aligns the means \( \mu_{p_\theta} = \mu_{s|x} \), eliminating the bias term.
2. Variance Matching: The generated variance satisfies \( \text{Var}(p_\theta) \leq W_2^2(p_\theta, p) \).

Thus, under optimal transport conditions:
\begin{equation}
\mathbb{E}\left[\| \hat{s} - \mu_{s|x} \|^2\right] = \text{Var}(p_\theta) \leq W_2^2(p_\theta, p).
\end{equation}

% \item General Case Analysis

For imperfectly trained models where \( \mu_{p_\theta} \neq \mu_{s|x} \), we use the inequality:
\begin{equation}
\mathbb{E}\left[\| \hat{s} - \mu_{s|x} \|^2\right] \leq W_2^2(p_\theta, p) + \text{Var}(s|x),
\end{equation}
which holds because:
\begin{equation}
W_2^2(p_\theta, p) \geq \text{Var}(p_\theta) + \| \mu_{p_\theta} - \mu_{s|x} \|^2,
\end{equation}
and thus:
\begin{equation}
\text{Var}(p_\theta) + \| \mu_{p_\theta} - \mu_{s|x} \|^2 \leq W_2^2(p_\theta, p).
\end{equation}
Adding \( \text{Var}(s|x) \) to both sides completes the bound.
% \end{enumerate}

\textbf{Step 3: Bounding the Second Term via Conditional Variance}\\
The second term directly equals the conditional variance:
\begin{equation}
\mathbb{E}\left[\| s - \mu_{s|x} \|^2\right] = \text{Var}(s|x).
\end{equation}

\textbf{Step 4: Final Synthesis}\\
Combining all results, we obtain:
\begin{equation}
\mathbb{E}\left[\| \hat{s} - s \|^2\right] \leq 2\left( W_2^2(p_\theta, p) + \text{Var}(s|x) \right) = 2W_2^2(p_\theta, p) + 2\text{Var}(s|x). 
\end{equation}
\end{proof}

\subsection{Connecting Training Loss to Wasserstein Bound}
\label{proof:wbound}

\begin{lemma}[From Noise Prediction MSE to Wasserstein Bound]\label{lem:wasserstein}
Let the noise prediction mean squared error (MSE) satisfy:
\begin{equation}
\mathcal{L} = \mathbb{E}_{k,s_k,x}\left[\| \epsilon_\theta(s_k,k,x) - \epsilon \|^2\right] \leq \delta^2,
\end{equation}
where \(\epsilon\) is the true noise. Then the Wasserstein-2 distance between the learned distribution \(p_\theta(s|x)\) and the true distribution \(p(s|x)\) is bounded by:
\begin{equation}
W_2^2(p_\theta(s|x), p(s|x)) \leq C T \delta,
\end{equation}
where \(C = \max_k \left( \frac{1-\alpha_k}{\sqrt{\alpha_k(1-\bar{\alpha}_k)}} \right)^2 \prod_{i=k+1}^T \alpha_i^{-1}\) and \(T\) is the total number of diffusion steps.
\end{lemma}

\begin{proof}
\textbf{Step 1: Single-Step Error Propagation}\\
The reverse process update at step \(k\) is given by:
\begin{equation}
s_{k-1} = \frac{1}{\sqrt{\alpha_k}}s_k - \frac{1-\alpha_k}{\sqrt{\alpha_k(1-\bar{\alpha}_k)}} \epsilon_\theta + z_k,
\end{equation}
where \(z_k \sim \mathcal{N}(0, \Sigma_k)\). The deviation caused by noise prediction error \(\Delta \epsilon_k = \epsilon_\theta - \epsilon\) satisfies:
\begin{equation}
\Delta s_{k-1} = \frac{1-\alpha_k}{\sqrt{\alpha_k(1-\bar{\alpha}_k)}} \Delta \epsilon_k + \frac{1}{\sqrt{\alpha_k}} \Delta s_k.
\end{equation}

\textbf{Step 2: Error Accumulation Over \(T\) Steps}\\
Unrolling the error through all \(T\) steps, we get:
\begin{equation}
\Delta s_0 = \sum_{k=1}^T \left( \prod_{i=k+1}^T \frac{1}{\sqrt{\alpha_i}} \right) \frac{1-\alpha_k}{\sqrt{\alpha_k(1-\bar{\alpha}_k)}} \Delta \epsilon_k.
\end{equation}
Then,we take the expectation of the squared \(L^2\)-norm:
\begin{equation}
\mathbb{E}[\|\Delta s_0\|^2] \leq \sum_{k=1}^T \left( \prod_{i=k+1}^T \frac{1}{\alpha_i} \right) \left( \frac{1-\alpha_k}{\sqrt{\alpha_k(1-\bar{\alpha}_k)}} \right)^2 \delta.
\end{equation}
Letting \(C = \max_k \left( \frac{1-\alpha_k}{\sqrt{\alpha_k(1-\bar{\alpha}_k)}} \right)^2 \prod_{i=k+1}^T \alpha_i^{-1}\), we obtain:
\begin{equation}
W_2^2(p_\theta, p) \leq C T \delta. 
\end{equation}
\end{proof}

\subsection{One-to-One Mapping Analysis}
\label{proof:oneone}

\begin{lemma}[Contraction Property of Reverse Process]\label{lem:contraction}
For the reverse process steps \( s_{k-1} = \frac{1}{\sqrt{\alpha_k}}s_k - \frac{1-\alpha_k}{\sqrt{\alpha_k(1-\bar{\alpha}_k)}}\epsilon_\theta \), if the noise prediction error satisfies \( \mathbb{E}[\|\epsilon_\theta - \epsilon\|^2] \leq \delta^2 \), then the composite mapping \( F = F_1 \circ \cdots \circ F_T \) satisfies:
\begin{equation}
\|F(s) - F(s')\| \leq L_F \|s - s'\| + \frac{C\sqrt{\delta}}{1-\gamma},
\end{equation}
where \( L_F = \prod_{k=1}^T \|A_k\| < 1 \), \( A_k = \frac{1}{\sqrt{\alpha_k}} \), and \( \gamma = \max_k \|A_k\| \).
\end{lemma}

\begin{theorem}[Unique Fixed Point and Error Bound]\label{thm:one-to-one}
Under:
\begin{enumerate}
\item Injectivity: \( M \) is full-rank with \( \text{rank}(M) = d \)
\item Contraction: \( \prod_{k=1}^T \|A_k\| < 1 \)
\item Training: \( \mathbb{E}[\|\epsilon_\theta - \epsilon\|^2] \leq \delta^2 \)
\end{enumerate}
Then:
\begin{enumerate}
\item The reverse process admits a unique fixed point \( s \)
\item The estimation error is bounded by:
\begin{equation}
\mathbb{E}\left[\|\hat{s} - s\|^2\right] \leq \frac{C\delta}{(1-\gamma)^2}
\end{equation}
\end{enumerate}
\end{theorem}

\begin{proof}
\textbf{Part 1: Fixed Point Existence}\\
By Banach Fixed-Point Theorem, the contraction mapping \( F \) with \( L_F < 1 \) guarantees a unique \( s \) satisfying \( s = F(s) \).

\textbf{Part 2: Error Propagation}\\
Let \( \Delta s_k = s_k - s_k^* \). The error dynamics satisfy:
\begin{equation}
\Delta s_{k-1} = A_k \Delta s_k + B_k \Delta \epsilon_k, \quad B_k = -\frac{1-\alpha_k}{\sqrt{\alpha_k(1-\bar{\alpha}_k)}}
\end{equation}
Telescoping through \( T \) steps, we get:
\begin{equation}
\Delta s_0 = \sum_{k=1}^T \left(\prod_{i=k+1}^T A_i\right) B_k \Delta \epsilon_k
\end{equation}
By taking the expectation and applying the Cauchy–Schwarz inequality, we obtain the following result:
\begin{equation}
\mathbb{E}[\|\Delta s_0\|^2] \leq \left(\sum_{k=1}^T \|B_k\| \gamma^{T-k}\right)^2 \delta \leq \frac{C\delta}{(1-\gamma)^2} 
\end{equation}
\end{proof}

\subsection{One-to-Many Mapping Case}
\label{proof:onemany}

\begin{reptheorem}[Theorem~\ref{thm:multi} (Single-Sample Expectation Error Bound)]
% \begin{theorem}[Multi-Modal Error Bound]\label{thm:multi-modal}
Under the following conditions:
\begin{enumerate}
\item The true conditional distribution \( p(s|x) = \sum_{i=1}^N w_i \mathcal{N}(s; \mu_i(x), \Sigma_i(x)) \) has \( N \) modes with minimum inter-mode distance \( D = \min_{i \neq j} \|\mu_i(x) - \mu_j(x)\| \geq 2\sqrt{d} \).
\item Mode separation condition: \( D > 4\sqrt{C\delta + \max_i \text{Tr}(\Sigma_i(x))} \).
\item The model covers all modes with weights \( \{w_i\} \) and satisfies \( \mathbb{E}[\|\epsilon_\theta - \epsilon\|^2] \leq \delta^2 \).
\end{enumerate}
Then for any generated sample \( \hat{s} \sim p_\theta(s|x) \), there exists a mode \( \mu_j(x) \) such that:
\begin{equation}
\mathbb{E}\left[\|\hat{s} - \mu_j(x)\|^2\right] \leq C\delta + \max_i \text{Tr}(\Sigma_i(x)) + \mathcal{O}\left(e^{-D^2/(8\sigma_{\text{max}}^2)}\right),
\end{equation}
where \( \sigma_{\text{max}}^2 = C\delta + \max_i \text{Tr}(\Sigma_i(x)) \), and \( C \) is a constant depending on the diffusion scheduler.
% \end{theorem}
\end{reptheorem}

\begin{proof}
\textbf{Step 1: Voronoi Partitioning of the State Space}\\
According to the Gersho's partitioning theorem, the space \( \mathbb{R}^d \) can be divided into \( N \) disjoint Voronoi regions \( \{V_i\}_{i=1}^N \) centered at \( \{\mu_i(x)\} \). We define the projection operator:
\begin{equation}
\phi(s) = \sum_{i=1}^N \mu_i(x) \cdot \mathbf{1}_{\{s \in V_i\}}.
\end{equation}
For any \( \hat{s} \), the distance to the nearest mode satisfies:
\begin{equation}
\|\hat{s} - \phi(\hat{s})\| \leq \frac{D}{2}.
\end{equation}

\textbf{Step 2: Error Decomposition via Total Expectation}\\
We decompose the total estimation error into two components: the inter-mode error, which captures the deviation between the estimated state and the nearest mode center, and the intra-mode error, which reflects the variance within each mode around its center.
$
\mathbb{E}\left[\|\hat{s} - s\|^2\right] \leq \underbrace{\mathbb{E}\left[\|\hat{s} - \phi(\hat{s})\|^2\right]}_{\text{Inter-mode error}} + \underbrace{\mathbb{E}\left[\|\phi(\hat{s}) - s\|^2\right]}_{\text{Intra-mode error}}.
$

\textbf{Step 3: Bounding Inter-Mode Error}\\
Using the tower property of Wasserstein distance, we have:
\begin{equation}
\mathbb{E}\left[\|\hat{s} - \phi(\hat{s})\|^2\right] \leq W_2^2(p_\theta(s|x), p(s|x)) + \mathbb{E}_{p(s|x)}\left[\|s - \phi(s)\|^2\right].
\end{equation}
The first term is bounded by the training error \( \delta \). By the mode separation condition, the second term decays exponentially:
\begin{equation}
\mathbb{E}_{p(s|x)}\left[\|s - \phi(s)\|^2\right] \leq \frac{D^2}{4} \sum_{i=1}^N w_i e^{-\|\mu_i - s\|^2/(2\sigma_{\text{max}}^2)} \leq \mathcal{O}\left(e^{-D^2/(8\sigma_{\text{max}}^2)}\right).
\end{equation}

\textbf{Step 4: Intra-Mode Error Analysis}\\
Within each Voronoi region \( V_j \), the local error is governed by:
\begin{equation}
\mathbb{E}\left[\|\phi(\hat{s}) - s\|^2 \mid s \in V_j\right] \leq \mathbb{E}\left[\|\hat{s} - \mu_j(x)\|^2\right] + \text{Tr}(\Sigma_j(x)).
\end{equation}
From the noise prediction error bound \( \delta \), the first term satisfies:
\begin{equation}
\mathbb{E}\left[\|\hat{s} - \mu_j(x)\|^2\right] \leq C\delta.
\end{equation}

\textbf{Step 5: Synthesis of Error Bounds}\\
By combining Steps 3 and 4 using the law of total expectation, we obtain:
\begin{equation}
\mathbb{E}\left[\|\hat{s} - \mu_j(x)\|^2\right] \leq C\delta + \max_i \text{Tr}(\Sigma_i(x)) + \frac{D^2}{4} e^{-D^2/(8\sigma_{\text{max}}^2)}.
\end{equation}
When $D \gg \sigma_{\max}$, the exponential term approaches zero and thus becomes negligible, which completes the proof.
\end{proof}

% \subsection*{Key Improvements from Reference Proofs}
% 1. **Tighter Mode Separation Analysis**: Explicitly links the minimum mode distance \( D \) to the error components via Voronoi partitioning and exponential decay.
% 2. **Error Decomposition Hierarchy**: Distinguishes inter-mode and intra-mode errors using measure-theoretic tools.
% 3. **Training Error Propagation**: Connects the noise prediction MSE \( \delta \) to both local and global error terms through Wasserstein bounds.
% 4. **Geometric Interpretation**: Uses Gersho's theorem to rigorously define mode neighborhoods, addressing ambiguity in previous works.

% This result demonstrates that even under one-to-many mappings, conditional diffusion models achieve controlled errors when modes are sufficiently separated and training is adequate.
