# Supplementary material for: GlobeDiff: State Diffusion Process for Partial Observability in Multi-Agent Systems
Source: arXiv:2602.15776 source file (2026-02-17)
Supplement: Supplementary file 3 [file limitation.tex]

\clearpage
\section{Limitations}
\label{lim}
Our method requires constructing a dataset using an offline pre-trained diffusion model. While this approach is effective in many cases, it may be less straightforward in complex environments where data collection is more challenging. First, it requires the availability of pre-collected data, which may not always be feasible, particularly in complex or dynamic environments. Moreover, suitable datasets may not be readily available for all scenarios of interest, which may limit the practical applicability and generalization of the proposed approach in certain complex environments.
